# Supplementary material for: TagMe: GPS-Assisted Automatic Object Annotation in Videos
Source: arXiv:2103.13428 source file (2021-03-24)
Supplement: Supplementary file 1 [file appendix-approach.tex]

\section{Details of \name\ Pipeline}
\subsection{Clustering Algorithm in Candidate Object Proposal Stage}
\label{appendix:dbscan-ac}
We use DBSCAN as our basic clustering algorithm. We find the basic DBSCAN algorithm works decently in most of the cases, however, it has two limitations,
\begin{compactenum}
    \item When two moving objects are very close to each other, they will be clustered into the same cluster. We show an example of this in Figure~\ref{afig:dbscan} (Basic DBSCAN).
    \item DB-SCAN algorithm has a distance threshold parameter. If the distance between two points is closer than this distance threshold, the two points are considered connected. We find using a single threshold cannot work well for both large (close to the camera) objects and small (far away from the camera) objects at the same time. 
\end{compactenum}

To address the first limitation, we introduce the \textit{affinity constraint} to the basic DBSCAN algorithm. We call this algorithm DBSCAN-AC. DBSCAN-AC takes temporal information into account so that it can prevent many objects being clustered into one big object, e.g., the examples shown in Figure~\ref{afig:dbscan}. The idea here is, if two optical flows were clustered into different clusters in many frames in the past, they are unlikely to be from the same object and should not be clustered into the same cluster even if they are close enough to each other. 

We implement the affinity constraint through maintaining the affinity scores between every two optical flows. If two optical flows are close enough to each other in one frame, we increase the affinity score by $1.0$. If two optical flows are not clustered into the same cluster, we decrease the affinity score by $0.5$. During clustering, we only consider the optical flow pairs whose affinity score is greater than $0$. We find this solution is quite effective - it can prevent many objects being clustered into one big object, e.g., the examples shown in Figure~\ref{afig:dbscan}. As a result, DBSCAN-AC can work well with a large distance threshold, which is necessary for large objects. 

\begin{figure}[h]
    \centering
    %\vspace{-0.3cm}
    \includegraphics[width=\linewidth]{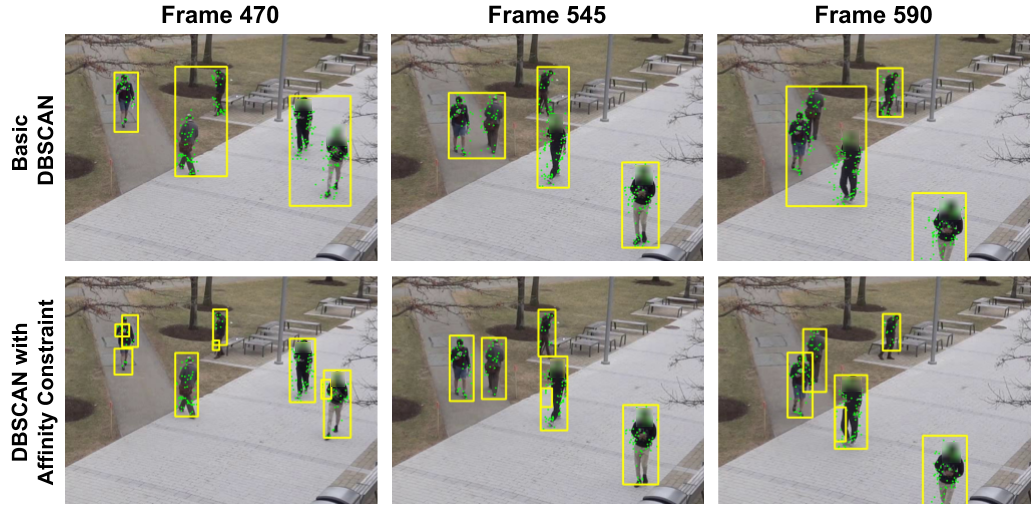}
    \caption{We show the clusters generated by the basic DBSCAN and DBSCAN-AC (with the same distance threshold) using yellow boxes. We show the moving optical flows as green dots. }
    \label{afig:dbscan}
\end{figure}

To address the second limitation, we combine the candidate objects generated with different DBSCAN distance thresholds. In our quantitative evaluation, we find combining the output from the basic DBSCAN with a small distance threshold (for small and far-away objects) and the output from DBSCAN-AC with a large distance threshold (for large and close objects) yields the best quality. Therefore, we use the candidate objects generated from this combination in the succeeding stages.
