# Supplementary material for: TagMe: GPS-Assisted Automatic Object Annotation in Videos
Source: arXiv:2103.13428 source file (2021-03-24)
Supplement: Supplementary file 2 [file appendix-evaluation.tex]

\section{Evaluation Details}
\subsection{Candidate Object Proposal}
\label{appendix:candidate-object-proposal}
We evaluate the quality of the generated candidate objects by comparing the bounding box of the best candidate object at each frame with the ground-truth in that frame. Here, at each frame, the best candidate object is the object which maximizes the IoU metric to the ground-truth. We report the statistics from the IoU metric and the Median-ND metric for different candidate object proposal methods. 

\begin{figure}[h]
    \centering
    %\vspace{-0.3cm}
    \includegraphics[width=\linewidth]{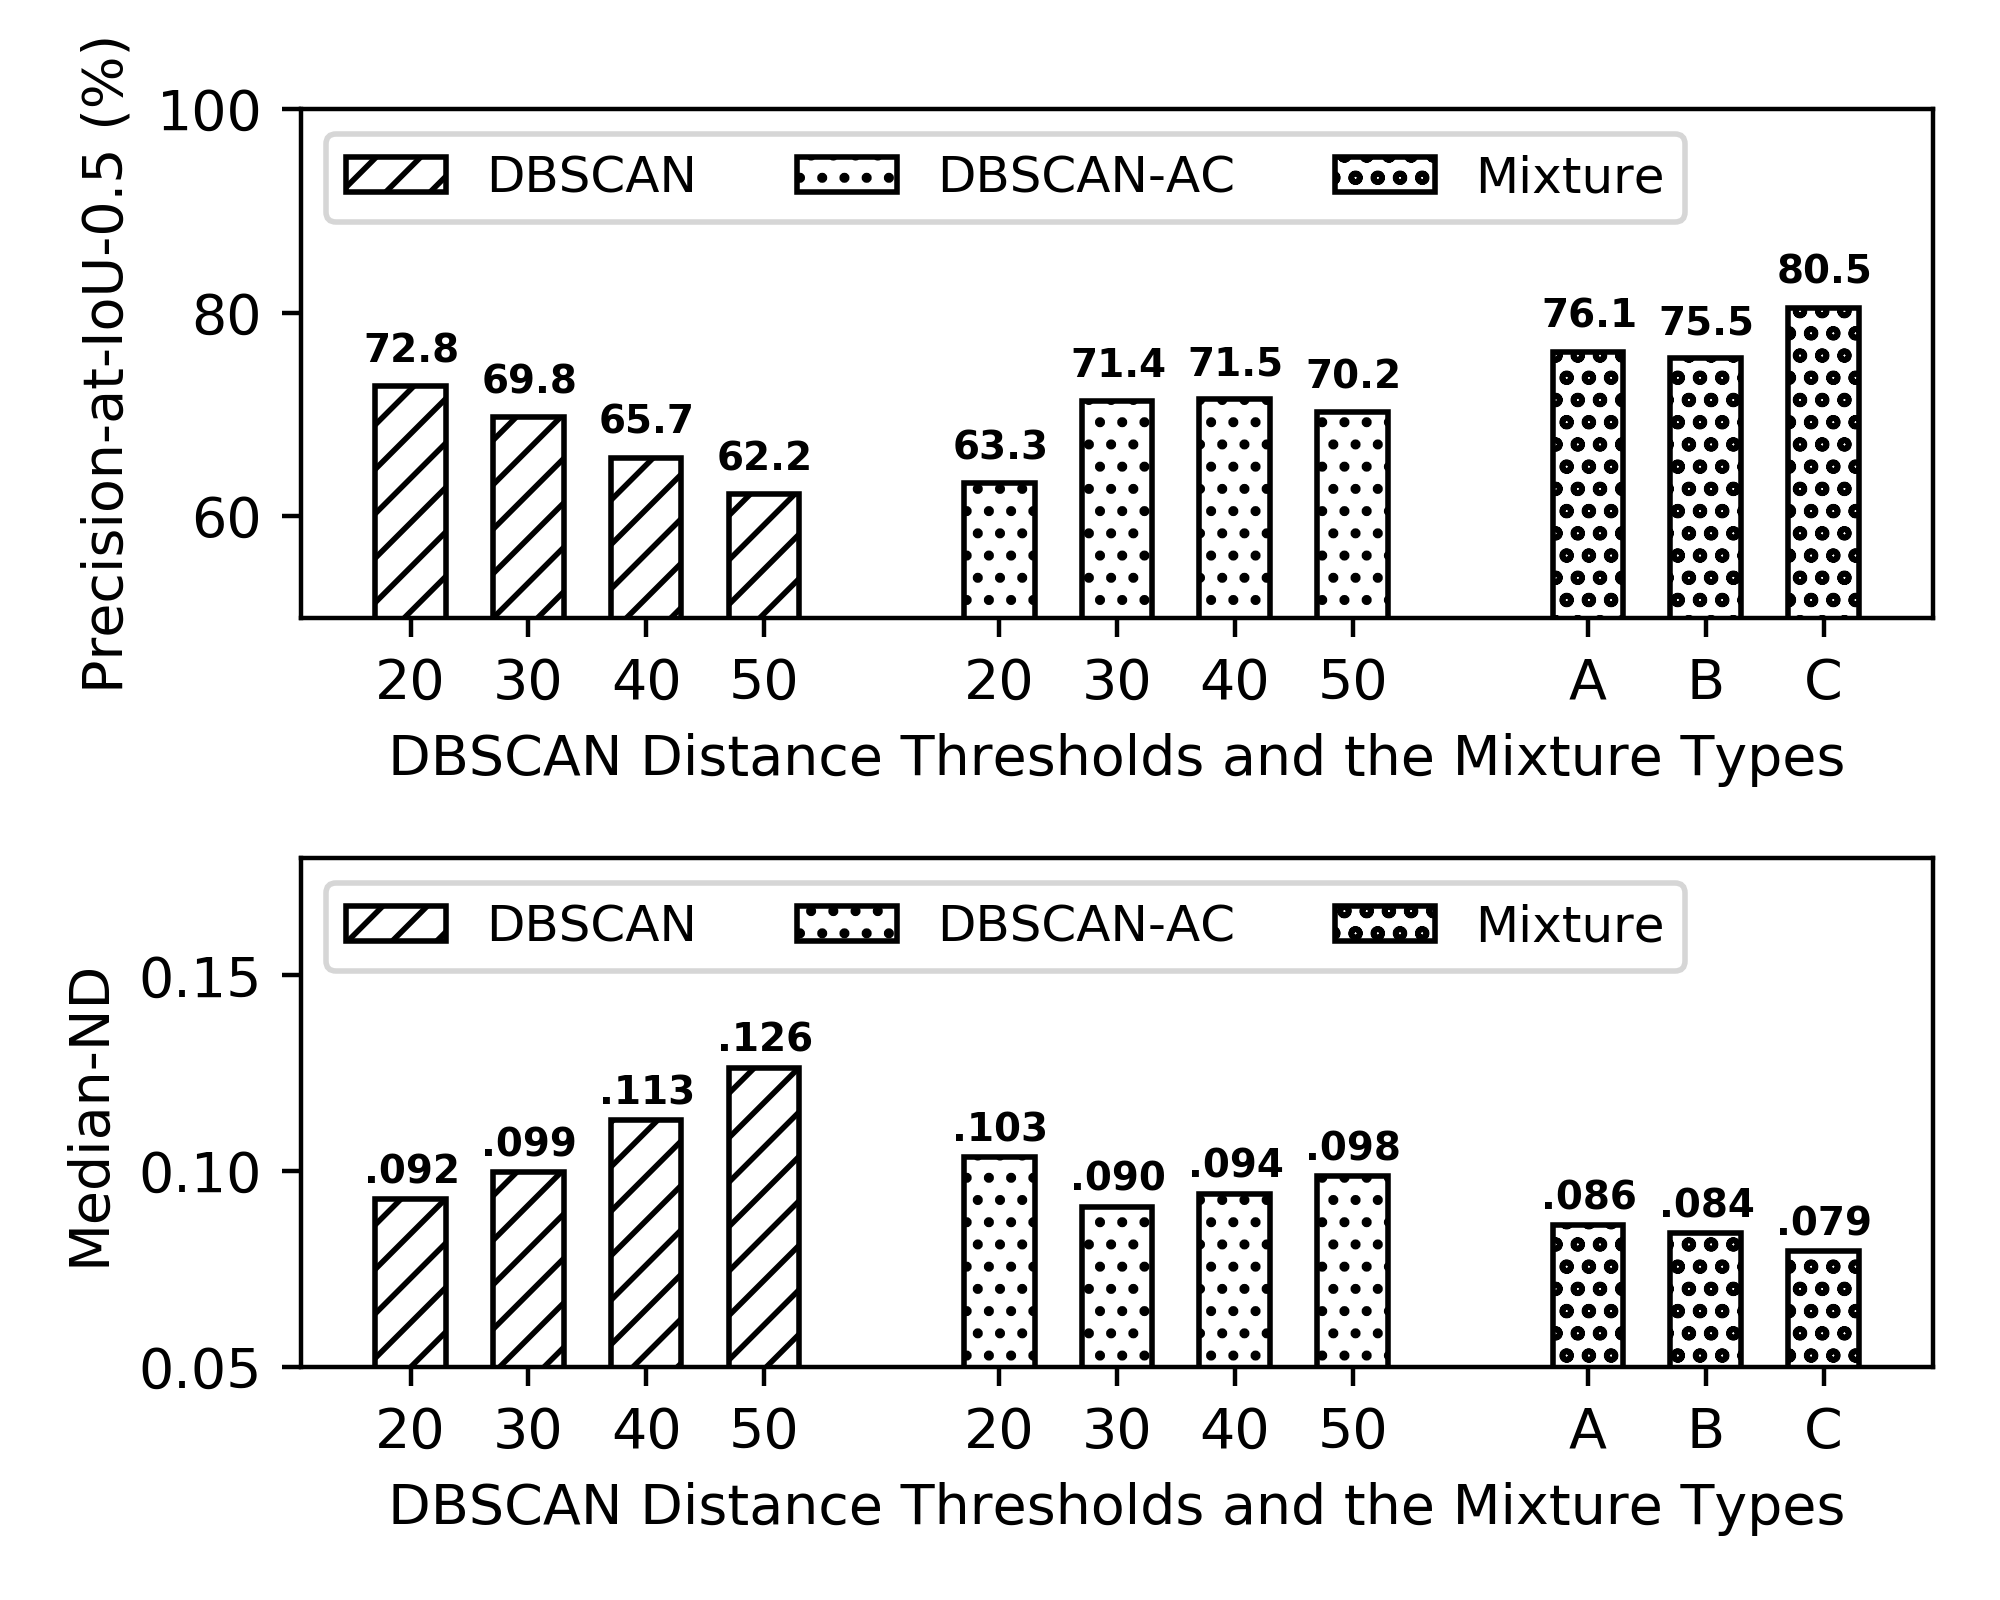}
    \vspace{-0.3cm}
    \caption{Quality of different candidate object proposal methods. }
    \label{fig:stage1}
    \vspace{-0.3cm}
\end{figure}

We show the precision-at-IoU-0.5 (higher is better) and the median normalized distance (lower is better) in Figure~\ref{fig:stage1}. We find the traditional DBSCAN approach performs well with small distance threshold (the unit is in pixel), however, it cannot scale well to larger distance thresholds which are necessary for larger objects. This is because when the distance threshold is large, DBSCAN may put two nearby objects into one cluster, therefore, it may generate many oversized bounding boxes that decrease the candidates' quality.

We addressed this scalability issue by introducing the \textit{affinity constraint} (DBSCAN-AC in  Figure~\ref{fig:stage1}), which allows DBSCAN to use larger distance thresholds, as a result, DBSCAN-AC can handle large objects.

As the distance thresholds are related to the object size, we combine the candidate objects generated with a small distance threshold, i.e., 20 pixels, for small objects, and a large distance threshold, i.e., 50 pixels, for large objects.

In Figure~\ref{fig:stage1}, we show the results from three mixtures. Mixture-A uses the candidates from the basic DBSCAN method, Mixture-B uses the candidates from DBSCAN-AC method, and Mixture-C uses the candidates from the basic DBSCAN method for small objects and the candidates from the DBSCAN-AC method for large objects. We find all three mixtures perform better than methods using only one distance threshold. Among the three mixtures, Mixture-C performs the best, therefore, we use it in our succeeding stages.

\subsection{Qualitative Results}
\label{appendix:qualitative-results}
We show examples of both good quality bounding boxes and bad quality bounding boxes produced by \name's first three stages, and the corresponding quality ranking (prediction result of Stage-4) in Figure~\ref{fig:goodsamples} and Figure~\ref{fig:badsamples}.   

We can find \name\ can produce many good quality bounding boxes that are sufficient in many training tasks. Although there are still some bad quality bounding boxes, they can be effectively excluded in the bounding box ranking stage (Stage-4). TagMe system is not designed to annotate all the video frames but to produce annotations in an opportunistic way. Because we assume that TagMe system is running continuously, even if we only create annotations for 1\% of the all video frames, that will be a huge amount of annotations per day.

\begin{figure*}[h]
    \centering
    %\vspace{-0.3cm}
    \includegraphics[width=1.0\linewidth]{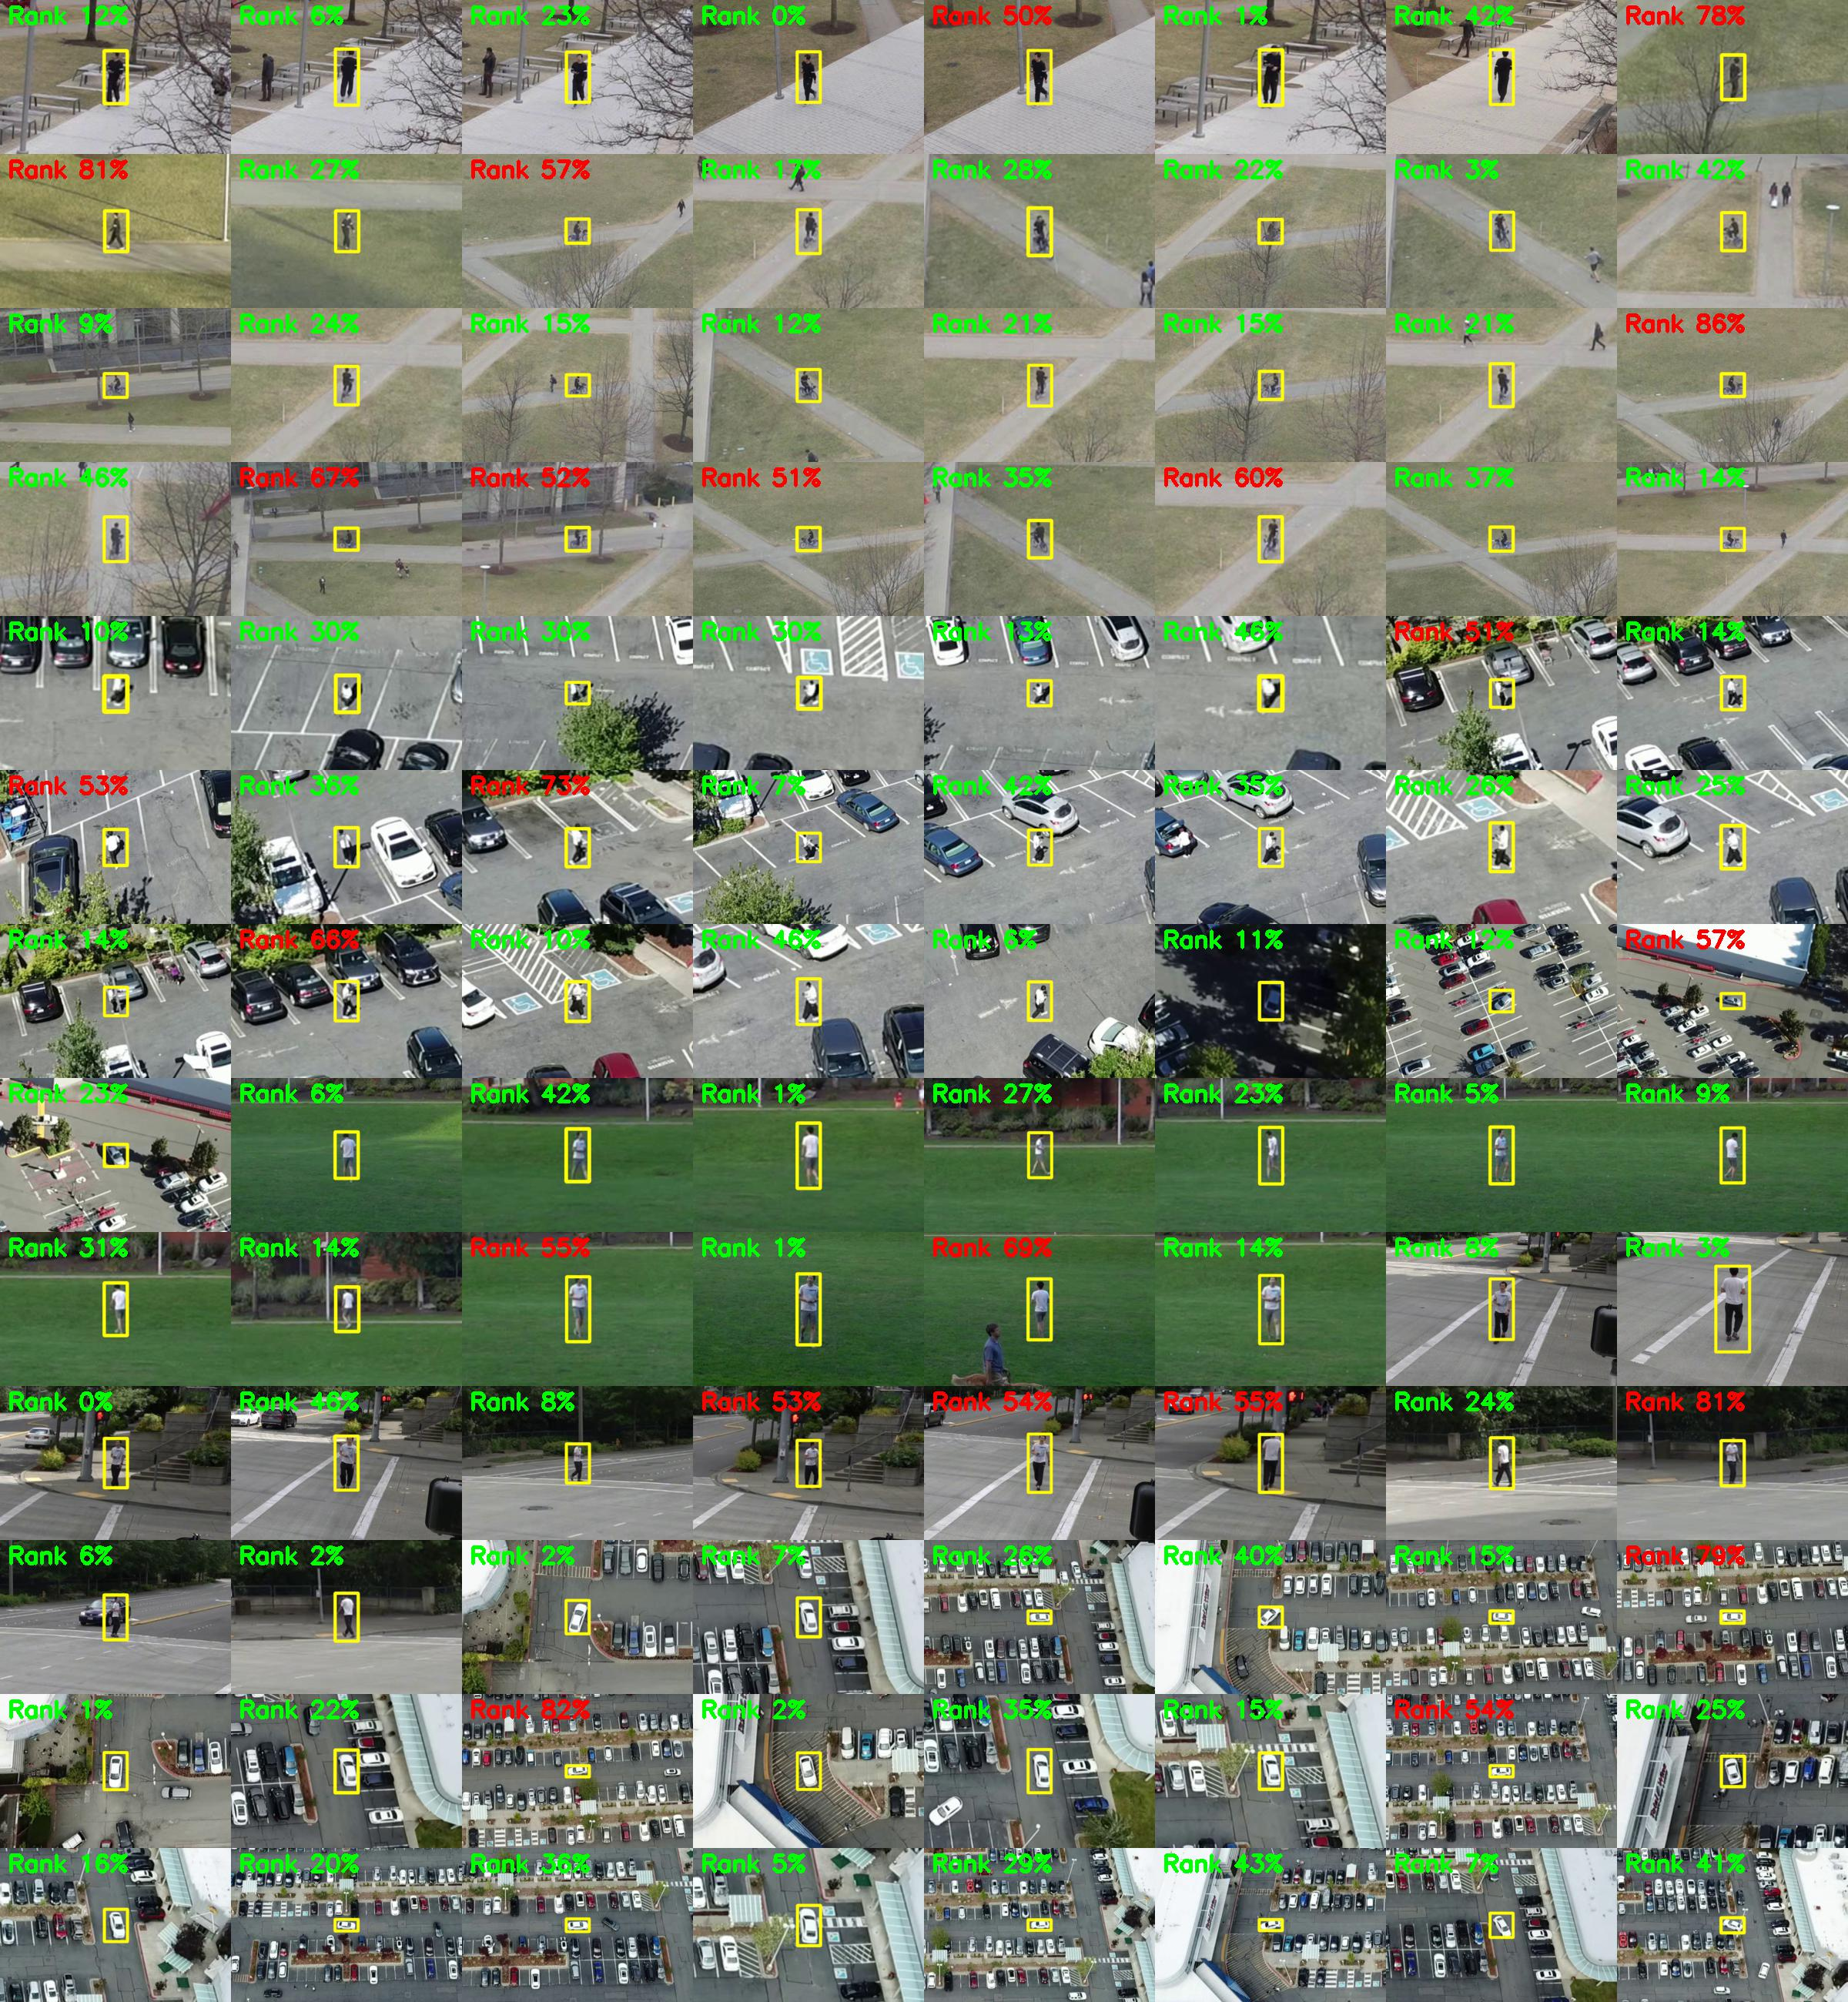}
    % \vspace{-0.3cm}
    \caption{Examples of good bounding boxes (i.e., IoU $>$ 0.85) produced by \name's first three stages. We show the corresponding quality ranking prediction (Stage-4) at the top-left corner in each image. Here, lower ranking number indicates better quality prediction. In each image, the text is green if the bounding box belongs to the top-50\% of the all bounding boxes. Otherwise, we draw the text in red. We can find most of the good quality bounding boxes have good quality ranking, therefore, most of them will not be excluded through bounding box ranking (Stage-4). }
    \vspace{-0.3cm}
    \label{fig:goodsamples}
\end{figure*}

\begin{figure*}[t!]
    %\centering
    %\vspace{-0.3cm}
    \includegraphics[width=\linewidth]{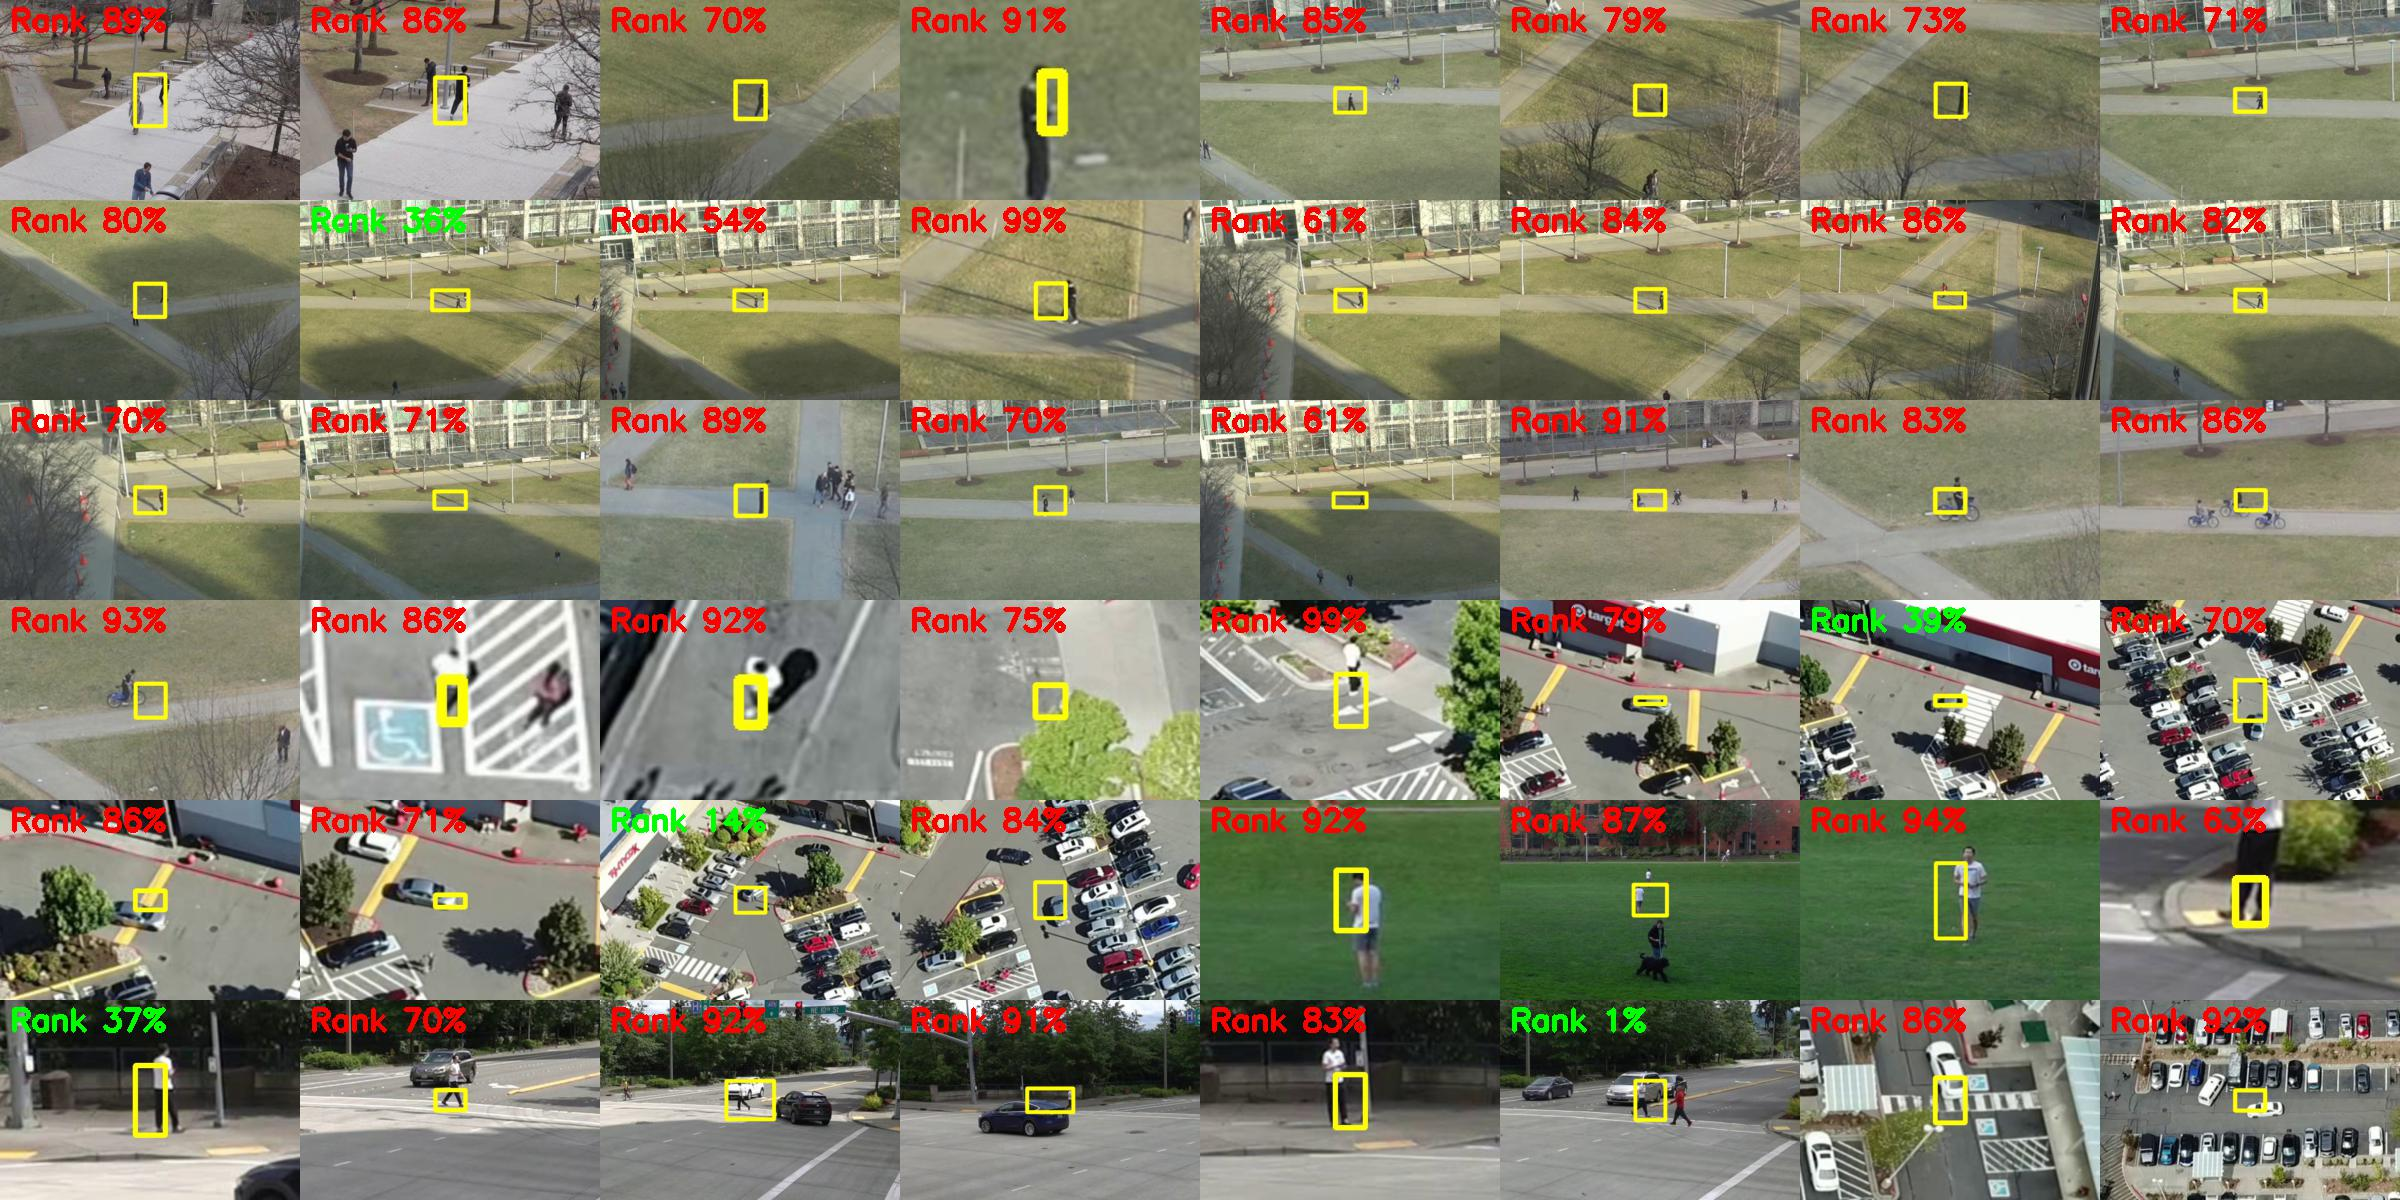}
    \caption{Examples of bad bounding boxes (i.e., IoU $<$ 0.3) produced by \name's first three stages. We show the corresponding quality ranking prediction (Stage-4) at the top-left corner in each image. Here, lower ranking number indicates better quality prediction. In each image, the text is green if the bounding box belongs to the top-50\% of the all bounding boxes. Otherwise, we draw the text in red. We can find many of the bad quality bounding boxes can be excluded through bounding box ranking (Stage-4). }
    \vspace{11.0cm}
    \label{fig:badsamples}
\end{figure*}
